# Supplementary material for: Efficiently Forgetting What You Have Learned in Graph Representation Learning via Projection
Source: arXiv:2302.08990 source file (2023-02-17)
Supplement: Supplementary file 1 [file discussion_on_privacy.tex]

\section{Some discussion on privacy and potential concerns} \label{section:some_random_discussion}

In this section, we give some discussion on the current stage of machine unlearning. This section can be think of is as an extension of the conclusion section (Section~\ref{section:conclusion}). We summarize the topic of each paragraph in boldface at the beginning of each paragraph.

\noindent\textbf{Different privacy measurement.}
Most of the existing machine unlearning literature are heavily relying on the definition of differential privacy. For example, one of the most widely accepted notation is \textit{certified removal}~\cite{guo2020certified}, which is defined as $\exp(-\epsilon) \leq P(\mathbf{w}_p) / P(\mathbf{w}_u) \leq \exp(\epsilon)$. Please notice that the certified notation shares the same spirit to our result in Theorem~\ref{theorem:ell2_norm_of_weight_projections} because both the model considered in ours and~\cite{guo2020certified} are linear and convex.
However, since~\cite{guo2020certified} is an approximate unlearning strategy by its nature, one cannot know whether the \textit{influence} of the deleted data is perfectly removed, therefore adding random noises to the weight parameters is required during the unlearning process.

\noindent\textbf{Different \textit{influence} definition.}
In fact, the definition of \textit{influence} is still not well defined and it is different from one literature to another.
Although different notations on \textit{influence} could be ambiguous, we believe each of them has its own value.
For example, \cite{guo2020certified} measures the \textit{influence} as the norm of a second-order gradient and they reduce such \textit{influence} by using single-step of  second-order gradient update. 
In this paper, we consider \textit{influence} as whether the learned weight parameters actually contain the deleted data. Therefore, we propose an unlearning strategy to project the original solution onto a subspace that is irrelevant to the deleted node features.

\noindent\textbf{An alternative view on our \textit{influence} definition.}
Let's suppose the original linear GNN model is trained by uniform mini-batch neighbor sampling. 
Since our key idea is to find a new solution from a subspace that does not contain the deleted data, 
one can think of \our as using importance mini-batch neighbor sampling to train on the dataset after node deletion, where the nodes that have higher similarity to the deleted nodes are sampled more frequently.

% \weilin{show some guarantees on privacy (e.g., based on assumptions you made that removed data can be approximated by remaining data)}

\noindent\textbf{Some other concern on subspace overlapping.}
A reader might have some concern on whether \our still work well if there exist an node feature that could be represented by any other node features, i.e., $\mathbf{x}_i \in \text{span}\{ \mathbf{x}_1, \ldots, \mathbf{x}_{i-1}, \mathbf{x}_{i+1}, \ldots, \mathbf{x}_n \}$.
Indeed, \our cannot $100\%$ remove the information of $\mathbf{x}_i$ from the learned weight parameters. 
In fact, we argue that such $\mathbf{x}_i$ is not necessarily removed as an adversary also cannot distinguish whether the information is from a single user's feature or a combination of multiple users' features.
However, for the completeness and to avoid the potential confusion, we propose to add some tiny random noise to all node features so that $\mathbf{x}_i \not\in \text{span}\{ \mathbf{x}_1, \ldots, \mathbf{x}_{i-1}, \mathbf{x}_{i+1}, \ldots, \mathbf{x}_n \}$.
