# Supplementary material for: Efficiently Forgetting What You Have Learned in Graph Representation Learning via Projection
Source: arXiv:2302.08990 source file (2023-02-17)
Supplement: Supplementary file 2 [file linear_as_expressive_as_nonlinear.tex]

\section{Linear-GNN is almost as powerful as non-linear counterparts} \label{section:linear_vs_unlearn_expressive}

In this section, we summarize recent studies~\cite{wei2022understanding,wang2022powerful} shows that linear-GNNs are almost as expressive as its non-linear counterparts.
Although two papers study from different perspective (i.e., \cite{wei2022understanding} studies from Bayesian inference and~\cite{wang2022powerful} studies from spectral neural network), they all lead to a similar conclusion that linear-GNNs are almost as expressive as its non-linear counterparts under some assumption on the node features and graph structure properties.

\subsection{From Bayesian inference perspective}
\cite{wei2022understanding} compares linear-GNN and non-linear GNN from the Bayesian inference perspective.
They consider binary node classification where the graph is randomly generated by contextual stochastic block models (CSBM).
They measure the success of node classification by signal-to-noise ratio (SNR).
They show that under some assumptions on the CSBM, the SNR of non-linear GNN is in the same order as linear-GNN.

More specifically,~\cite{wei2022understanding} assumes the random graphs are generated by contextual stochastic block models (CSBM), where each node has a feature vector $\mathbf{x}_i \in \mathbb{R}^m$ and a binary category label $y_i \in \{+1,-1\}$.
Let us suppose $\mathcal{G}(\mathcal{V},\mathcal{E})$ is an graph generated by $\text{CSBM}(n,p,q,\mathbb{P}_{+1}, \mathbb{P}_{-1})$ with the following processes: 
\begin{itemize}
    \item (Generate node labels) For each node $v_i \in \mathcal{V}$, we randomly sample the label from $y_i \in \{+1,-1\}$, where $n=|\mathcal{V}|$ is the number of nodes.
    \item (Generate graph structure) If any two nodes have the same label $y_i = y_j$, then with probability $p$ we add edge $(v_i, v_j)$ to the edge set $\mathcal{E}$. Otherwise, with probability $q$  we add edge $(v_i, v_j)$ to the edge set $\mathcal{E}$.
    \item (Generate node features) If a node $y_i=+1$, then its feature vector $\mathbf{x}_i$ is sampled from $\mathbb{P}_{+1} = \mathcal{N}(\bm{\mu}_{+1}, \mathbf{I}/m)$. Otherwise, if a node $y_i=-1$, then its feature vector $\mathbf{x}_i$ is sampled from $\mathbb{P}_{-1} = \mathcal{N}(\bm{\mu}_{-1}, \mathbf{I}/m)$.
\end{itemize}

After that,~\cite{wei2022understanding} formulates non-linear GNN and linear-GNN under the context of Bayesian inference, where the optimal propagation is derived from max-a-posterior estimation.
To classify a node $v_i$, the optimal non-linear propagation is defined as
\begin{equation}
    \mathcal{P}_i = \psi(\mathbf{x}_i) + \sum_{j\in\mathcal{N}(v_i)} \phi(\psi(\mathbf{x}_j); \log(p/q)),
\end{equation}
where $\psi(\mathbf{x}) = \log(\mathbb{P}_{+1}(\mathbf{x}) / \mathbb{P}_{-1}(\mathbf{x}))$ and $\phi(\psi, \log(p/q)) = \text{ReLU}(\psi + \log(p/q)) - \text{ReLU}(\psi - \log(p/q)) - \log(p/q)$.
Similarly, for linear-GNN, the optimal linear propagation is defined as
\begin{equation}
    \mathcal{P}^l_i(\alpha) = \psi^\prime(\mathbf{x}_i) + \alpha \sum_{j\in\mathcal{N}(v_i)} \psi^\prime (\mathbf{x}_j),
\end{equation}
where $\psi^\prime(\mathbf{x}) = m \times \left( \langle\bm{\mu}_{+1} - \bm{\mu}_{-1}, \mathbf{x} \rangle - (\| \bm{\mu}_{+1} \|_2^2 - \| \bm{\mu}_{+1} \|_2^2) / 2 \right) $ and $\alpha$ is a parameter to balance information from the root node and its neighbors.

The minimal Bayesian mis-classification error is measured by signal-to-noise ratio (SNR), which is defined as $\rho$ for non-linear GN and $\rho_l$ for linear-GNN, 
\begin{equation}
    \rho = \frac{(\mathbb{E}[\mathcal{P}_i|y_i = +1] - \mathbb{E}[\mathcal{P}_i|y_i = -1])^2}{\text{variance}(\mathcal{P}_i | y_i = +1)},~
    \rho_l = \max_\alpha \frac{(\mathbb{E}[\mathcal{P}^l_i(\alpha)|y_i = +1] - \mathbb{E}[\mathcal{P}^l_i(\alpha)|y_i = -1])^2}{\text{variance}(\mathcal{P}_i^l(\alpha) | y_i = +1)}.
\end{equation}

They make the following assumptions on the random graph generator CSBM.
More specifically,~\cite{wei2022understanding} assumes the graph structure generated by $p,q$ is neither too strong (e.g., $p\rightarrow 1$ and $q\rightarrow 0$) or too weak (e.g., graph is too sparse) in Assumption~\ref{assumption:wang_graph_not_too_strong} assumes feature generation distributions for positive nodes and negative nodes are not too different.

\begin{assumption} [Assumption on graph structure] \label{assumption:wang_graph_not_too_strong}
Let us define $\mathcal{S}(p,q) = (p-q)^2/(p+q)$. They assume no very weak graph structure information $\mathcal{S}(p,q) = \omega_n \left( (\log n)^2 / n \right)$ and no very strong graph structure information $\mathcal{S}(p,q) \not\rightarrow |p-q|$.
\end{assumption}

\begin{assumption} [Assumption on node features] \label{assumption:wang_feats_not_too_strong}
Recall that $\bm{\mu}_{+1}$ is the mean of positive node feature distribution and $\bm{\mu}_{-1}$ is the mean of negative node feature distribution. Then, we assume  $\sqrt{m} \| \bm{\mu}_{+1} - \bm{\mu}_{-1}\|_2 = \mathcal{O}_n(1)$
\end{assumption}

Then,~\cite{wei2022understanding} has the following conclusion on the SNR of linear-GNN and non-liear GNN. In particular, they show that non-linear GNN behaves similar to the linear-GNN as their SNRs are in the same order.
In other word, under some assumption on graph structure and node features, the linear-GNN could be as expressive as non-linear GNN.

\begin{theorem} [Theorem 2 part 1 of~\cite{wei2022understanding}]
If CSBM satisfy Assumption~\ref{assumption:wang_graph_not_too_strong} and Assumption~\ref{assumption:wang_feats_not_too_strong}, we have $\rho_r = \Theta_n(\rho_l)$.
\end{theorem}

\noindent\textbf{When non-linearity is helpful?}
Besides, they show that non-linearity is helpful only if the Assumption~\ref{assumption:wang_feats_not_too_strong} does not hold. In other word, if the mean of the positive and negative node feature sampling distribution is different enough $\sqrt{m} \| \bm{\mu}_{+1} - \bm{\mu}_{-1}\|_2 = \omega_n(1)$, then $\rho_r = \omega_n(\rho_l)$.

\subsection{From spectral neural network perspective}

\cite{wang2022powerful} shows that linear-GNNs could produce arbitrary predictions under mild conditions on the Laplacian and node features, without relying on the non-linearity in MLP. 
The expressive power of linear-GNNs mainly comes from its weighted combination of multi-hop graph convolution operators.

Let us define $\mathbf{L} \in \mathbb{R}^{n\times n}$ as the Laplacian matrix in spectral GNNs, where $\mathbf{U}$ is the eigenvectors of $\mathbf{L}$ and $\mathbf{\Lambda}$ is the diagonal matrix of eigenvalues. They make the following assumptions on $\mathbf{L}$.

\begin{assumption} [Assumption on $\mathbf{L}$] \label{assumption:eigen_values}
    No eigenvalues of $\mathbf{L}$ are identical.
\end{assumption}

Let us denote $\mathbf{X}\in\mathbb{R}^{n\times d}$ as the node features and $\Tilde{\mathbf{X}} = \mathbf{U} \mathbf{X}$ as the graph Fourier transform of node features $\mathbf{X}$.
They make the following assumption on $\Tilde{\mathbf{X}}$.
\begin{assumption} [Assumption on $\Tilde{\mathbf{X}}$] \label{assumption:node_signal}
    No rows of $\Tilde{\mathbf{X}}$ are zero vector.
\end{assumption}

Given any target function $\mathbf{z} = f(\mathbf{L}, \mathbf{X}) \in \mathbb{R}^{n\times 1}$ we want to approximate via linear-GNN.
\cite{wang2022powerful} shows that there exists a linear-GNN can approximate function $f(\mathbf{L}, \mathbf{X})$ arbitrary close if Assumption~\ref{assumption:eigen_values} and Assumption~\ref{assumption:node_signal} hold. 
\begin{theorem}
Let us define $g_{\bm{\alpha}, \mathbf{w}}(\mathbf{L}, \mathbf{X}) = \sum_{\ell=1}^k \alpha_\ell \mathbf{L}^\ell \mathbf{X} \mathbf{w} $ as the linear-GNN and $f$ is the target function we want to approximate. Under the Assumption~\ref{assumption:eigen_values} and Assumption~\ref{assumption:node_signal}, there is always exists a set of $\bm{\alpha}^\star \in\mathbb{R}^k, \mathbf{w}^\star \in \mathbb{R}^d$ such that $g_{\bm{\alpha}^\star, \mathbf{w}^\star}(\mathbf{L}, \mathbf{X}) = f(\mathbf{L}, \mathbf{X})$. 
\end{theorem}

In practice, \cite{wang2022powerful} found Assumption~\ref{assumption:eigen_values} and Assumption~\ref{assumption:node_signal} are very likely to hold on the real-world datasets. 

\noindent\textbf{When non-linearity is helpful?}
They show that adding non-linear MLP to linear-GNNs could alleviate the conditions on node features (i.e., Assumption~\ref{assumption:node_signal}) because the output of multi-layer neural network are very likely to satisfy this condition. However, adding non-linearity will not necessarily improve its expressive power if the conditions are already satisfied in the first place.
