# Supplementary material for: Efficiently Forgetting What You Have Learned in Graph Representation Learning via Projection
Source: arXiv:2302.08990 source file (2023-02-17)
Supplement: Supplementary file 3 [file link_pred.tex]

\section{Graph representation unlearning for link prediction}\label{section:link_pred}
In this section, we study the application of \our on the link prediction down stream task on the OGB-Collab dataset.

\noindent\textbf{Setup.}
In OGB-Collab link prediction dataset, each node is associated with node feature vector $\mathbf{x}_i$. 
The link representation of a node pair $(v_i, v_j)$ is computed as $\mathbf{e}_{ij} = \mathbf{h}_i \odot \mathbf{h}_j$, where $\mathbf{h}_i = [\mathbf{P} \mathbf{X}]_i$ is the node representation of the node $i$.
Given the whether a link exists in a subset of node pairs, our goal is to predict whether a link exist in the rest of the node pairs.
The model performance is evaluated by ranking each true collaboration among a set of 100K randomly-sampled negative collaborations, and count the ratio of positive edges that are ranked at 50-place or above (Hits@50).

\subsection{Feature-label injection test}

Similar to the \textit{feature-label injection test} for node classification, we add an extra-label category to the dataset and all deleted nodes are changed to this extra-label category. Then, we append an extra binary feature to all nodes, set the extra binary feature as \textit{one} for the deleted nodes and as \textit{zero} for other nodes, and pre-train on the modified dataset.
The effectiveness of unlearning method is evaluated by comparing the norm of weight parameters of the extra-feature channel before and after the unlearning process.
For linear GNN, we expect the weight norm of this extra-feature channel greater than zero before unlearning due to the strong correlation between the extra feature-label, however, the value is expected to be zero after unlearning because such correlation no long exists in the dataset.
The deleted nodes is randomly selected as $2\%, 5\%, 10\%$ of the nodes from the training set.

As shown in Table~\ref{table:feature_injection_test}, 
% we have the following observations: (1) By comparing the weight norm before and after unlearning, we know that \our and  \textsc{GraphEraser} can perfectly unlearn the correlation between the extra-feature and label by setting the extra-feature channel as zero, however, \textsc{Influence}+ and \textsc{Fisher}+ still have part of the information left in the weight; (2) By comparing the wall-clock time, \our has a lower computation cost and requires less time to unlearn, especially when comparing to \textsc{GraphEraser}; (3) By observing the accuracy of \textsc{Influence}+ and \textsc{Fisher}+, these approaches suffers performance degradation because a stronger regularization is required to stabilize the unlearning process, which will dominates the loss; (4) By comparing the performance of \our with and without adaptive diffusion, we know that adaptive diffusion provides consistent performance boosting to linear GNN models.

\begin{table}[H]
\centering
\caption{Comparison on the \textcolor{brown}{ Hits@50},
% the number of the delete nodes that are predicted as the extra-label category (\textcolor{cyan}{Num delete}),
the norm of extra-feature weight channel (\textcolor{cyan}{Weight norm}) before and after unlearning (denoted as \textit{before} $\rightarrow$ \textit{after}), and wall-clock time (\textcolor{teal}{Time}) using linear GNN. 
% ``-'' stands for cannot generate meaningful results.
}
\label{table:feature_injection_test_link_pred}
\scalebox{0.8}{
\begin{tabular}{l l l l l l}
\hline\hline \rule{0pt}{2ex}   
                                       & Method                & Metrics  & Delete $2\%$ nodes           & Delete $5\%$ nodes           & Delete $10\%$ nodes        \\ \hline\hline \rule{0pt}{2ex}   
\multirow{12}{*}{\rotatebox[origin=c]{90}{\textbf{OGB-Collab}}}    
                                       & \cellcolor[HTML]{FEDEDC} & \cellcolor[HTML]{FEDEDC}\textcolor{brown}{Accuracy}      & \cellcolor[HTML]{FEDEDC}$73.39\rightarrow 73.32$       & \cellcolor[HTML]{FEDEDC}$73.33\rightarrow 73.39$       & \cellcolor[HTML]{FEDEDC}$73.25\rightarrow 73.39$     \\ 
                                       & \cellcolor[HTML]{FEDEDC} & \cellcolor[HTML]{FEDEDC}\textcolor{cyan}{Weight norm}    & \cellcolor[HTML]{FEDEDC}$19.4\rightarrow 0$   & \cellcolor[HTML]{FEDEDC}$21.7 \rightarrow 0$  & \cellcolor[HTML]{FEDEDC}$56.8 \rightarrow 0$\\
                                       & \cellcolor[HTML]{FEDEDC} \multirow{-3}{*}{\our}  & \cellcolor[HTML]{FEDEDC}\textcolor{teal}{Time}      & \cellcolor[HTML]{FEDEDC}$0.07$ s      & \cellcolor[HTML]{FEDEDC}$0.07$ s    & \cellcolor[HTML]{FEDEDC} $0.07$ s    \\ \cline{2-6} \rule{0pt}{2ex}   
                                       %%%%%%%%%%%%%%%%%%%%%%%%%%%%%%%%%%%%%%%%%%%%%%%%%%%%%%%%%%%%%%%%%%%%%%%%%%%%%%%%%%%%%%%%%%%%%%%%%%%%%%%%%%%%%%%%%%%%%%%%%%%%%%%%%%%%%%%%%%%%
                                       %%%%%%%%%%%%%%%%%%%%%%%%%%%%%%%%%%%%%%%%%%%%%%%%%%%%%%%%%%%%%%%%%%%%%%%%%%%%%%%%%%%%%%%%%%%%%%%%%%%%%%%%%%%%%%%%%%%%%%%%%%%%%%%%%%%%%%%%%%%%
                                       %%%%%%%%%%%%%%%%%%%%%%%%%%%%%%%%%%%%%%%%%%%%%%%%%%%%%%%%%%%%%%%%%%%%%%%%%%%%%%%%%%%%%%%%%%%%%%%%%%%%%%%%%%%%%%%%%%%%%%%%%%%%%%%%%%%%%%%%%%%%
                                       & \cellcolor[HTML]{C4F8F6} & \cellcolor[HTML]{C4F8F6}\textcolor{brown}{Accuracy}         & \cellcolor[HTML]{C4F8F6}$73.44\rightarrow 73.52$         & \cellcolor[HTML]{C4F8F6}$73.42\rightarrow 73.48$         & \cellcolor[HTML]{C4F8F6}$73.34\rightarrow 73.44$     \\ 
                                       & \cellcolor[HTML]{C4F8F6} & \cellcolor[HTML]{C4F8F6}\textcolor{cyan}{Weight norm}  & \cellcolor[HTML]{C4F8F6}$21.0\rightarrow 0$ & \cellcolor[HTML]{C4F8F6}$24.3 \rightarrow 0$  & \cellcolor[HTML]{C4F8F6}$25.6 \rightarrow 0$ \\
                                       & \cellcolor[HTML]{FEDEDC} \multirow{-3}{*}{\cellcolor[HTML]{C4F8F6}\begin{tabular}[c]{@{}l@{}} \our \\ (+ adapt diff) \end{tabular}}    & \cellcolor[HTML]{C4F8F6}\textcolor{teal}{Time}      & \cellcolor[HTML]{C4F8F6}$0.07$ s      & \cellcolor[HTML]{C4F8F6}$0.07$ s    & \cellcolor[HTML]{C4F8F6}$0.07$ s \\ \cline{2-6} \rule{0pt}{2ex}  
                                       %%%%%%%%%%%%%%%%%%%%%%%%%%%%%%%%%%%%%%%%%%%%%%%%%%%%%%%%%%%%%%%%%%%%%%%%%%%%%%%%%%%%%%%%%%%%%%%%%%%%%%%%%%%%%%%%%%%%%%%%%%%%%%%%%%%%%%%%%%%%
                                       %%%%%%%%%%%%%%%%%%%%%%%%%%%%%%%%%%%%%%%%%%%%%%%%%%%%%%%%%%%%%%%%%%%%%%%%%%%%%%%%%%%%%%%%%%%%%%%%%%%%%%%%%%%%%%%%%%%%%%%%%%%%%%%%%%%%%%%%%%%%
                                       %%%%%%%%%%%%%%%%%%%%%%%%%%%%%%%%%%%%%%%%%%%%%%%%%%%%%%%%%%%%%%%%%%%%%%%%%%%%%%%%%%%%%%%%%%%%%%%%%%%%%%%%%%%%%%%%%%%%%%%%%%%%%%%%%%%%%%%%%%%%
                                       & \multirow{3}{*}{\textsc{GraphEraser}} 
                                                               & \textcolor{brown}{Accuracy}      & $63.41\rightarrow 63.39$       & $63.41\rightarrow 63.38$       & $63.41\rightarrow 63.36$      \\ 
                                       &                       & \textcolor{cyan}{Weight norm ($\times 10^{-3}$)}    & $8.8 \rightarrow 0$   & $8.8 \rightarrow 0$   & $8.8 \rightarrow 0$ \\
                                       &                       & \textcolor{teal}{Time}           & $112.1$ s   & $112.1$ s   & $112.1$ s \\\cline{2-6} \rule{0pt}{2ex}    
                                       %%%%%%%%%%%%%%%%%%%%%%%%%%%%%%%%%%%%%%%%%%%%%%%%%%%%%%%%%%%%%%%%%%%%%%%%%%%%%%%%%%%%%%%%%%%%%%%%%%%%%%%%%%%%%%%%%%%%%%%%%%%%%%%%%%%%%%%%%%%%
                                       %%%%%%%%%%%%%%%%%%%%%%%%%%%%%%%%%%%%%%%%%%%%%%%%%%%%%%%%%%%%%%%%%%%%%%%%%%%%%%%%%%%%%%%%%%%%%%%%%%%%%%%%%%%%%%%%%%%%%%%%%%%%%%%%%%%%%%%%%%%%
                                       %%%%%%%%%%%%%%%%%%%%%%%%%%%%%%%%%%%%%%%%%%%%%%%%%%%%%%%%%%%%%%%%%%%%%%%%%%%%%%%%%%%%%%%%%%%%%%%%%%%%%%%%%%%%%%%%%%%%%%%%%%%%%%%%%%%%%%%%%%%%
                                       & \multirow{3}{*}{\textsc{Influence}+} 
                                                              & \textcolor{brown}{Accuracy}      & $63.39\rightarrow 63.39$       & $63.39\rightarrow 63.26$       & $63.39\rightarrow 63.07$      \\ 
                                       &                       & \textcolor{cyan}{Weight norm ($\times 10^{-3}$)}    & $12.6 \rightarrow 11.6$   & $12.6 \rightarrow 10.1$   & $12.6 \rightarrow 7.3$ \\
                                       &                       & \textcolor{teal}{Time}           & $0.8$ s   & $0.8$ s   & $0.8$ s \\\cline{2-6} \rule{0pt}{2ex}    
                                    %   %%%%%%%%%%%%%%%%%%%%%%%%%%%%%%%%%%%%%%%%%%%%%%%%%%%%%%%%%%%%%%%%%%%%%%%%%%%%%%%%%%%%%%%%%%%%%%%%%%%%%%%%%%%%%%%%%%%%%%%%%%%%%%%%%%%%%%%%%%%%
                                    %   %%%%%%%%%%%%%%%%%%%%%%%%%%%%%%%%%%%%%%%%%%%%%%%%%%%%%%%%%%%%%%%%%%%%%%%%%%%%%%%%%%%%%%%%%%%%%%%%%%%%%%%%%%%%%%%%%%%%%%%%%%%%%%%%%%%%%%%%%%%%
                                    %   %%%%%%%%%%%%%%%%%%%%%%%%%%%%%%%%%%%%%%%%%%%%%%%%%%%%%%%%%%%%%%%%%%%%%%%%%%%%%%%%%%%%%%%%%%%%%%%%%%%%%%%%%%%%%%%%%%%%%%%%%%%%%%%%%%%%%%%%%%%%
                                      & \multirow{3}{*}{\textsc{Fisher}+} 
                                                              & \textcolor{brown}{Accuracy}      & $63.39\rightarrow 63.56$       & $63.39\rightarrow 63.57$       & $63.39\rightarrow 63.57$      \\ 
                                       &                       & \textcolor{cyan}{Weight norm ($\times 10^{-3}$)}    & $12.6 \rightarrow 60.5$   & $12.6 \rightarrow 60.5$   & $12.6 \rightarrow 60.7$ \\
                                       &                       & \textcolor{teal}{Time}           & $1.2$ s   & $1.2$ s   & $1.2$ s \\\cline{2-6} \rule{0pt}{2ex}        
\end{tabular}
}
\vspace{-3mm}
\end{table}

% influence based training time: 
% retraining linear GNN 1,335 sec
