# Supplementary material for: Efficiently Forgetting What You Have Learned in Graph Representation Learning via Projection
Source: arXiv:2302.08990 source file (2023-02-17)
Supplement: Supplementary file 4 [file nonlinear.tex]

\subsection{An Unlearning Favorable Extension from Linear- to Non-linear GNN} \label{section:extension_non_linear}

In the following, we introduce a potential \textsc{Projector}-unlearning favorable extension to leverage the non-linearity in neural network architecture.

\noindent\textbf{Main insight.}
The geometric view of solving the logistic regression (as defined in Eq.~\ref{eq:ovr_logistic_regression}) is finding a hyperplane to linearly separate the node representation $\mathbf{H}$ computed by linear GNN. However, node representations might not be linearly separable. 
To overcome this issue, one could first apply an \textit{non-linear MLP} on each node features, 
then apply graph convolutions onto the output of the MLP before classification.
% , e.g., replacing the initialization of $\smash{\mathbf{h}_i^{(0)}}$  as $\smash{\mathbf{h}_i^{(0)} = \sigma (\mathbf{x}_i \mathbf{W}^{(1)}) \mathbf{W}^{(2)}}$ if using a $2$-layer MLP.
This can be interpreted as finding a non-linear separation in the input space. 
We note that our extension to non-linear is different from most non-linear GNN structure where an activation function and weight parameter matrix is used at each layer.
For example, if using a MLP with two weight matrices, the node representation is computed by the first row of the following equation, which is different from ordinary GNNs in the second row:
\begin{equation}
    \begin{aligned}
    \mathbf{H} &= \mathbf{P}^L \sigma(\sigma(\mathbf{X} \mathbf{W}^{(1)}_\text{mlp}) \mathbf{W}^{(2)}_\text{mlp}) \mathbf{W}^{(3)}_\text{gnn} & \text{Our proposal}\\
    \mathbf{H} &= \mathbf{P} \sigma( \mathbf{P} \sigma( \mathbf{P}\mathbf{X} \mathbf{W}^{(1)}_\text{gnn}) \mathbf{W}^{(2)}_\text{gnn}) \mathbf{W}^{(3)}_\text{gnn} & \text{Ordinary non-linear GNN}
    \end{aligned}
\end{equation}
% , e.g., the forward propagation rule in~\cite{kipf2016semi} as $\mathbf{H}^{(\ell)} = \sigma(\mathbf{P} \mathbf{H}^{(\ell-1)} \mathbf{W}^{(\ell)})$.
In our case, although the \emph{input} of MLP is relatively non-linear to each other, the \emph{output} of MLP is still relatively linear to each other, which allows us to utilize \our if MLP model is known not carrying the deleted node feature information.

\noindent\textbf{Non-linear extension.}
We propose to first pre-train the non-linear GNN on a public dataset with training samples that do not need to be forgotten, then we only need to take care of the data removal from the linear model that is applied to the output of the MLP.
By doing so, \our enjoys both the separation power brought by the non-linearity of MLP and the efficiency brought by the projection-based unlearning. For completeness, we conduct some preliminary experiments on the OGB-Arxiv and OGB-Product datasets by comparing the performance of non-linear GNNs to linear GNNs, where the MLP extractor is pre-trained on all node features except the deleted ones by supervised learning.
As shown in Table~\ref{table:linear_gnn_with_its_non_linear_extension}, we have the following observations: \circled{1} Although using MLP as a feature extractor can slightly improve the average F1-score accuracy, it also increases the variance of the model performance. \circled{2} Linear GNN could achieve better performance than ordinary GNNs by carefully tuning the hyper-parameters and using the label reuse tricks~\cite{wang2021bag}. \circled{3} Employing \textsc{GraphEraser} with non-linear GNNs will significantly hurt the performance of the original GNN models, which is due to the data heterogeneously and the lack of training data for each subgraph model. Such an observation  is aligned with the result originally reported in~\cite{chen2021graph} for mean-average prediction aggregation.

\input{tables/table_linear_gnn_with_mlp}
