# Supplementary material for: Efficiently Forgetting What You Have Learned in Graph Representation Learning via Projection
Source: arXiv:2302.08990 source file (2023-02-17)
Supplement: Supplementary file 5 [file robusness_projector.tex]

% \noindent\textbf{Robustness of \oure.}
\subsection{Robustness of \oure} \label{section:robustness}
We study the change of testing accuracy as we progressively increase the unlearning ratio from $1\%$ to $20\%$ chose the test accuracy of re-training ordinary GNNs from scratch as the baselines. A more stable model performance is more preferred in real-world scenarios as the model performance after unlearning is consistent with lower variance.
As shown in Figure~\ref{fig:test_perf}, the change of testing accuracy in \our is smaller (e.g., on OGB-Arvix dataset the test accuracy of \our changes around $0.5\%$ while the GNNs changes around $0.8\%\sim1\%$ ) and more stable (i.e., the test accuracy fluctuate less when the fraction of unlearning nodes increases) than re-training ordinary GNNs. Besides, linear GNNs achieve compatible or even better performance than non-linear counterparts, which motivates us rethink the expressive power of linear GNN against ordinary GNNs.
% Coupled with some peculiar properties of linear GNNs (e.g., convexity), which makes the choice of unlearning on linear structures as a good choice.
\begin{figure}[h]
    \centering
    % \vspace{-4mm}
    \includegraphics[width=\textwidth]{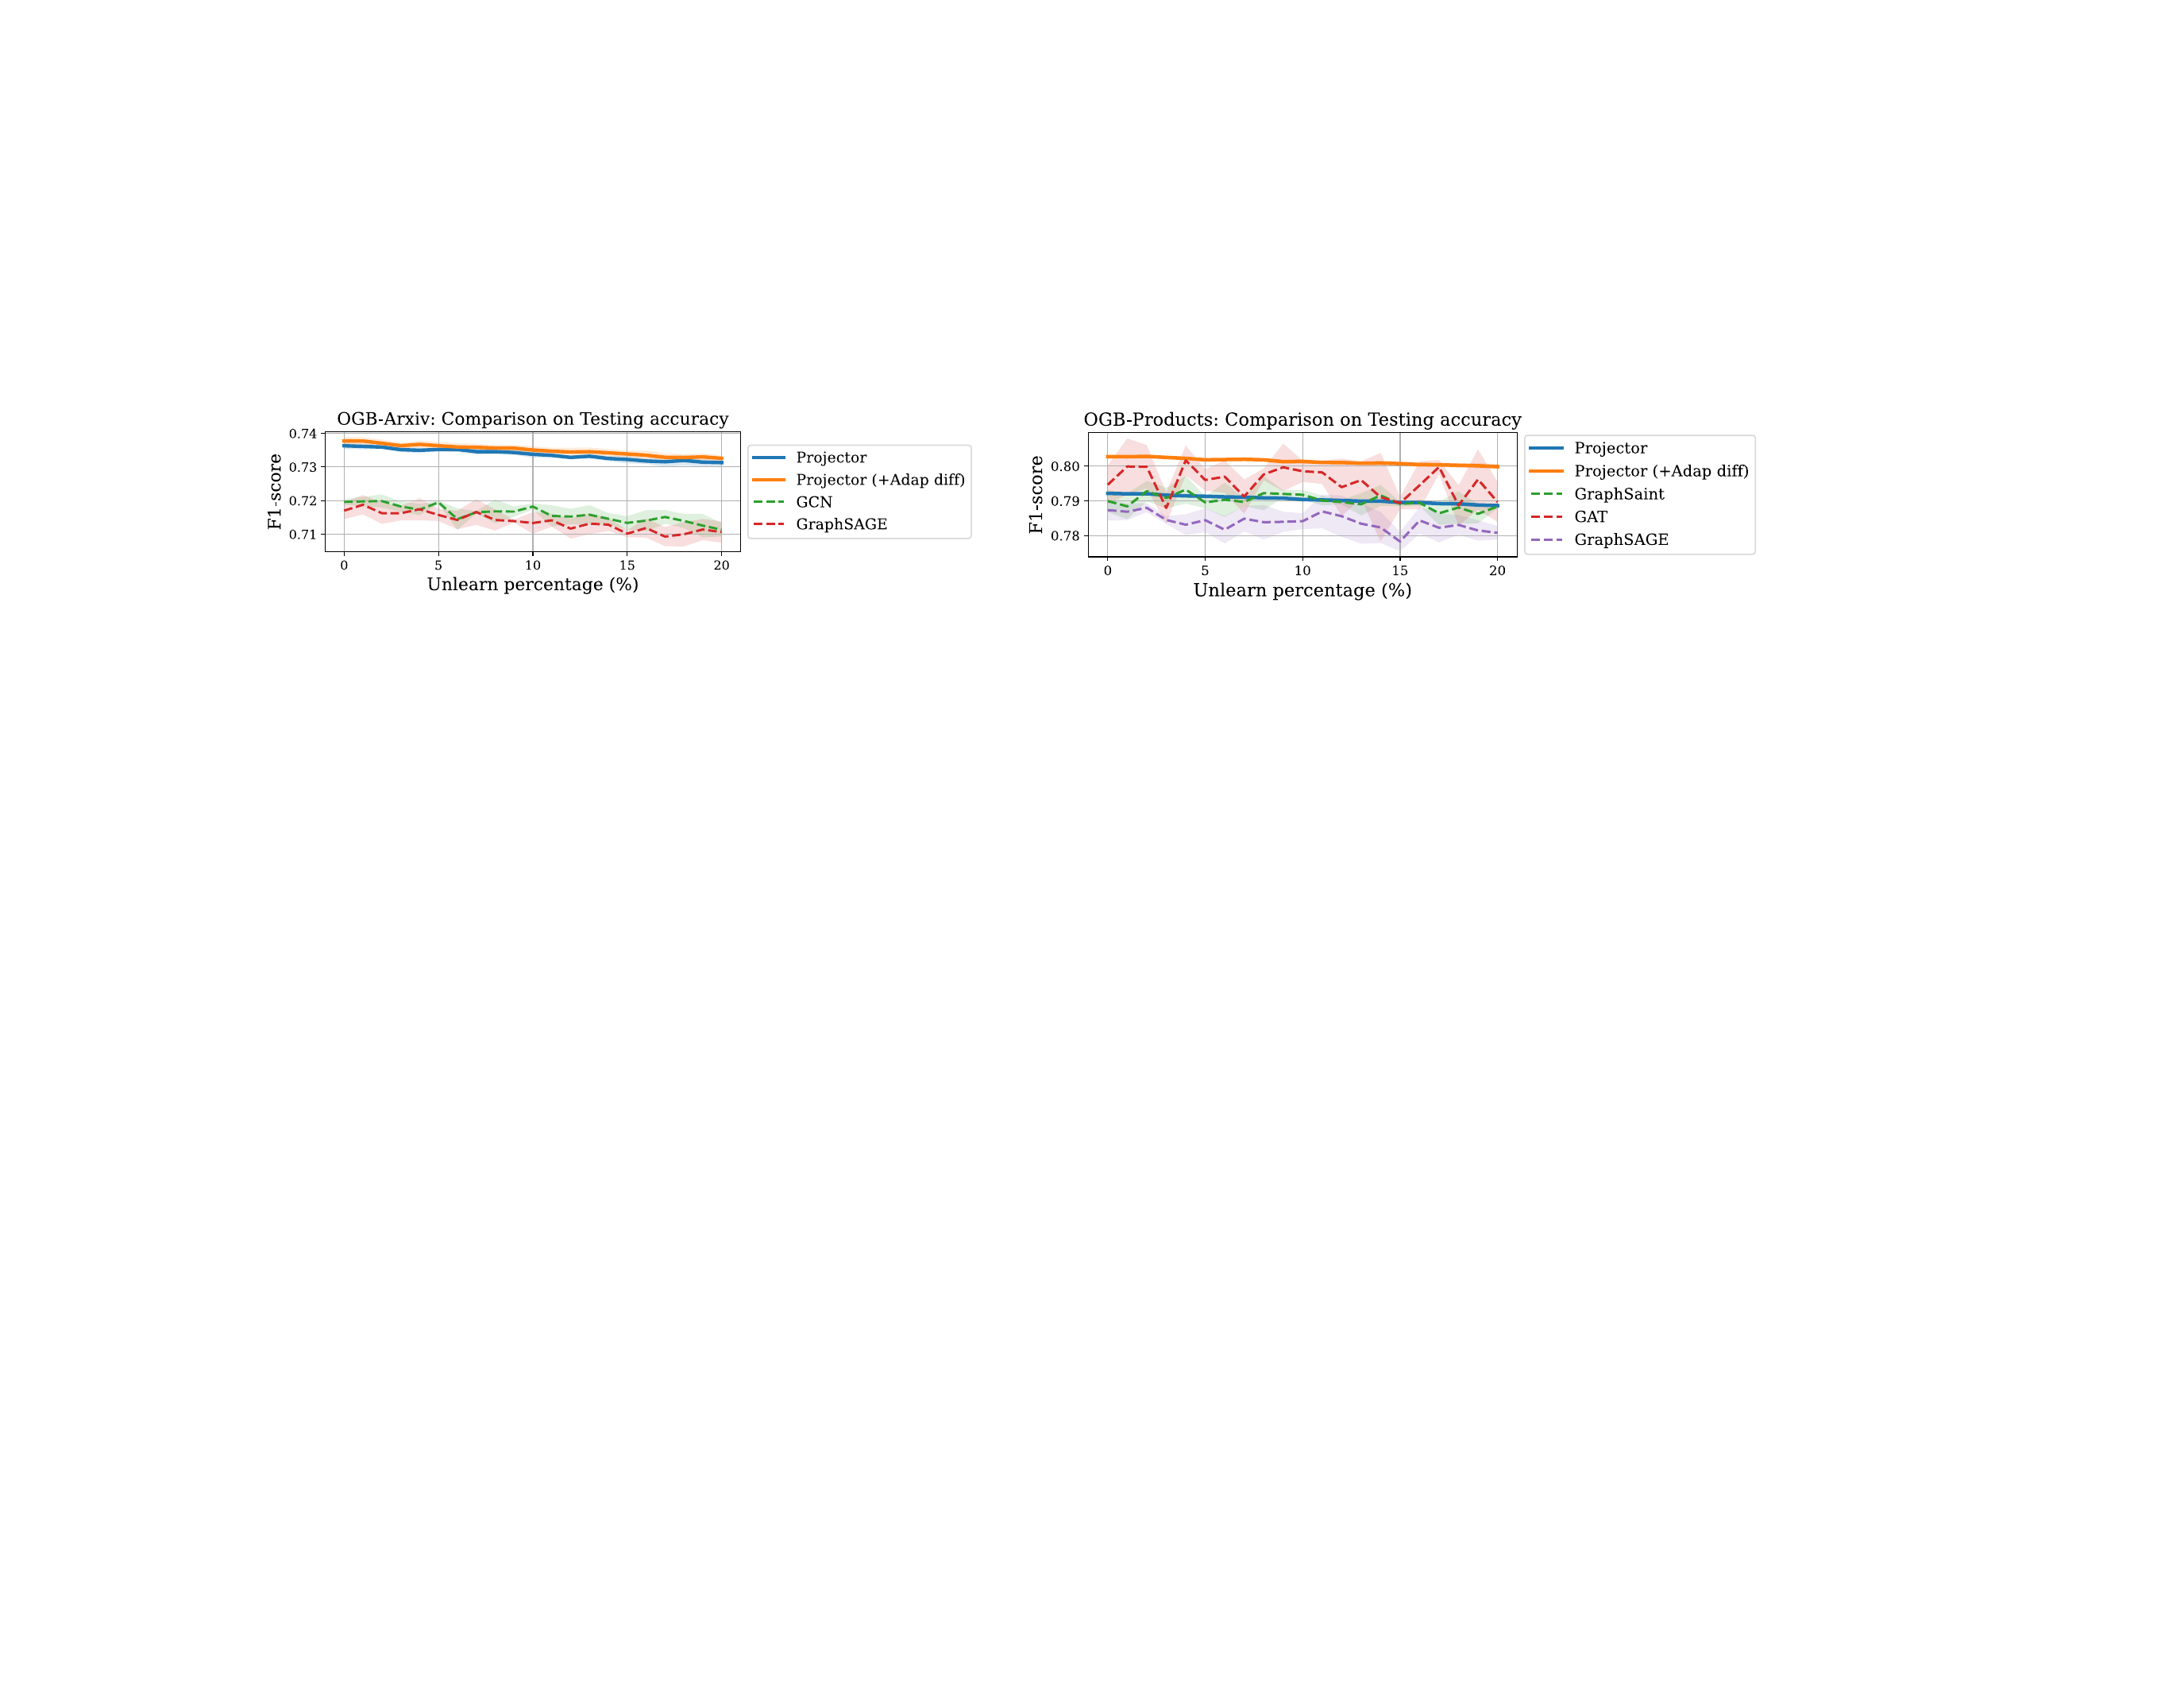}
    \vspace{-6mm}
    \caption{Comparison on the test performance with different number of node to unlearn. }
    \label{fig:test_perf}
    \vspace{-2mm}
\end{figure}
