# Supplementary material for: Efficiently Forgetting What You Have Learned in Graph Representation Learning via Projection
Source: arXiv:2302.08990 source file (2023-02-17)
Supplement: Supplementary file 6 [file feat_label_inject_link_pred.tex]

\begin{table}[H]
\centering
\caption{Comparison on the \textcolor{brown}{ Hits@50},
% the number of the delete nodes that are predicted as the extra-label category (\textcolor{cyan}{Num delete}),
the norm of extra-feature weight channel (\textcolor{cyan}{Weight norm}) before and after unlearning (denoted as \textit{before} $\rightarrow$ \textit{after}), and wall-clock time (\textcolor{teal}{Time}) using linear GNN. 
% ``-'' stands for cannot generate meaningful results.
}
\label{table:feature_injection_test_link_pred}
\scalebox{0.8}{
\begin{tabular}{l l l l l l}
\hline\hline \rule{0pt}{2ex}   
                                       & Method                & Metrics  & Delete $2\%$ nodes           & Delete $5\%$ nodes           & Delete $10\%$ nodes        \\ \hline\hline \rule{0pt}{2ex}   
\multirow{12}{*}{\rotatebox[origin=c]{90}{\textbf{OGB-Collab}}}    
                                       & \cellcolor[HTML]{FEDEDC} & \cellcolor[HTML]{FEDEDC}\textcolor{brown}{Accuracy}      & \cellcolor[HTML]{FEDEDC}$73.39\rightarrow 73.32$       & \cellcolor[HTML]{FEDEDC}$73.33\rightarrow 73.39$       & \cellcolor[HTML]{FEDEDC}$73.25\rightarrow 73.39$     \\ 
                                       & \cellcolor[HTML]{FEDEDC} & \cellcolor[HTML]{FEDEDC}\textcolor{cyan}{Weight norm}    & \cellcolor[HTML]{FEDEDC}$19.4\rightarrow 0$   & \cellcolor[HTML]{FEDEDC}$21.7 \rightarrow 0$  & \cellcolor[HTML]{FEDEDC}$56.8 \rightarrow 0$\\
                                       & \cellcolor[HTML]{FEDEDC} \multirow{-3}{*}{\our}  & \cellcolor[HTML]{FEDEDC}\textcolor{teal}{Time}      & \cellcolor[HTML]{FEDEDC}$0.07$ s      & \cellcolor[HTML]{FEDEDC}$0.07$ s    & \cellcolor[HTML]{FEDEDC} $0.07$ s    \\ \cline{2-6} \rule{0pt}{2ex}   
                                       %%%%%%%%%%%%%%%%%%%%%%%%%%%%%%%%%%%%%%%%%%%%%%%%%%%%%%%%%%%%%%%%%%%%%%%%%%%%%%%%%%%%%%%%%%%%%%%%%%%%%%%%%%%%%%%%%%%%%%%%%%%%%%%%%%%%%%%%%%%%
                                       %%%%%%%%%%%%%%%%%%%%%%%%%%%%%%%%%%%%%%%%%%%%%%%%%%%%%%%%%%%%%%%%%%%%%%%%%%%%%%%%%%%%%%%%%%%%%%%%%%%%%%%%%%%%%%%%%%%%%%%%%%%%%%%%%%%%%%%%%%%%
                                       %%%%%%%%%%%%%%%%%%%%%%%%%%%%%%%%%%%%%%%%%%%%%%%%%%%%%%%%%%%%%%%%%%%%%%%%%%%%%%%%%%%%%%%%%%%%%%%%%%%%%%%%%%%%%%%%%%%%%%%%%%%%%%%%%%%%%%%%%%%%
                                       & \cellcolor[HTML]{C4F8F6} & \cellcolor[HTML]{C4F8F6}\textcolor{brown}{Accuracy}         & \cellcolor[HTML]{C4F8F6}$73.44\rightarrow 73.52$         & \cellcolor[HTML]{C4F8F6}$73.42\rightarrow 73.48$         & \cellcolor[HTML]{C4F8F6}$73.34\rightarrow 73.44$     \\ 
                                       & \cellcolor[HTML]{C4F8F6} & \cellcolor[HTML]{C4F8F6}\textcolor{cyan}{Weight norm}  & \cellcolor[HTML]{C4F8F6}$21.0\rightarrow 0$ & \cellcolor[HTML]{C4F8F6}$24.3 \rightarrow 0$  & \cellcolor[HTML]{C4F8F6}$25.6 \rightarrow 0$ \\
                                       & \cellcolor[HTML]{FEDEDC} \multirow{-3}{*}{\cellcolor[HTML]{C4F8F6}\begin{tabular}[c]{@{}l@{}} \our \\ (+ adapt diff) \end{tabular}}    & \cellcolor[HTML]{C4F8F6}\textcolor{teal}{Time}      & \cellcolor[HTML]{C4F8F6}$0.07$ s      & \cellcolor[HTML]{C4F8F6}$0.07$ s    & \cellcolor[HTML]{C4F8F6}$0.07$ s \\ \cline{2-6} \rule{0pt}{2ex}  
                                       %%%%%%%%%%%%%%%%%%%%%%%%%%%%%%%%%%%%%%%%%%%%%%%%%%%%%%%%%%%%%%%%%%%%%%%%%%%%%%%%%%%%%%%%%%%%%%%%%%%%%%%%%%%%%%%%%%%%%%%%%%%%%%%%%%%%%%%%%%%%
                                       %%%%%%%%%%%%%%%%%%%%%%%%%%%%%%%%%%%%%%%%%%%%%%%%%%%%%%%%%%%%%%%%%%%%%%%%%%%%%%%%%%%%%%%%%%%%%%%%%%%%%%%%%%%%%%%%%%%%%%%%%%%%%%%%%%%%%%%%%%%%
                                       %%%%%%%%%%%%%%%%%%%%%%%%%%%%%%%%%%%%%%%%%%%%%%%%%%%%%%%%%%%%%%%%%%%%%%%%%%%%%%%%%%%%%%%%%%%%%%%%%%%%%%%%%%%%%%%%%%%%%%%%%%%%%%%%%%%%%%%%%%%%
                                       & \multirow{3}{*}{\textsc{GraphEraser}} 
                                                               & \textcolor{brown}{Accuracy}      & $63.41\rightarrow 63.39$       & $63.41\rightarrow 63.38$       & $63.41\rightarrow 63.36$      \\ 
                                       &                       & \textcolor{cyan}{Weight norm ($\times 10^{-3}$)}    & $8.8 \rightarrow 0$   & $8.8 \rightarrow 0$   & $8.8 \rightarrow 0$ \\
                                       &                       & \textcolor{teal}{Time}           & $112.1$ s   & $112.1$ s   & $112.1$ s \\\cline{2-6} \rule{0pt}{2ex}    
                                       %%%%%%%%%%%%%%%%%%%%%%%%%%%%%%%%%%%%%%%%%%%%%%%%%%%%%%%%%%%%%%%%%%%%%%%%%%%%%%%%%%%%%%%%%%%%%%%%%%%%%%%%%%%%%%%%%%%%%%%%%%%%%%%%%%%%%%%%%%%%
                                       %%%%%%%%%%%%%%%%%%%%%%%%%%%%%%%%%%%%%%%%%%%%%%%%%%%%%%%%%%%%%%%%%%%%%%%%%%%%%%%%%%%%%%%%%%%%%%%%%%%%%%%%%%%%%%%%%%%%%%%%%%%%%%%%%%%%%%%%%%%%
                                       %%%%%%%%%%%%%%%%%%%%%%%%%%%%%%%%%%%%%%%%%%%%%%%%%%%%%%%%%%%%%%%%%%%%%%%%%%%%%%%%%%%%%%%%%%%%%%%%%%%%%%%%%%%%%%%%%%%%%%%%%%%%%%%%%%%%%%%%%%%%
                                       & \multirow{3}{*}{\textsc{Influence}+} 
                                                              & \textcolor{brown}{Accuracy}      & $63.39\rightarrow 63.39$       & $63.39\rightarrow 63.26$       & $63.39\rightarrow 63.07$      \\ 
                                       &                       & \textcolor{cyan}{Weight norm ($\times 10^{-3}$)}    & $12.6 \rightarrow 11.6$   & $12.6 \rightarrow 10.1$   & $12.6 \rightarrow 7.3$ \\
                                       &                       & \textcolor{teal}{Time}           & $0.8$ s   & $0.8$ s   & $0.8$ s \\\cline{2-6} \rule{0pt}{2ex}    
                                    %   %%%%%%%%%%%%%%%%%%%%%%%%%%%%%%%%%%%%%%%%%%%%%%%%%%%%%%%%%%%%%%%%%%%%%%%%%%%%%%%%%%%%%%%%%%%%%%%%%%%%%%%%%%%%%%%%%%%%%%%%%%%%%%%%%%%%%%%%%%%%
                                    %   %%%%%%%%%%%%%%%%%%%%%%%%%%%%%%%%%%%%%%%%%%%%%%%%%%%%%%%%%%%%%%%%%%%%%%%%%%%%%%%%%%%%%%%%%%%%%%%%%%%%%%%%%%%%%%%%%%%%%%%%%%%%%%%%%%%%%%%%%%%%
                                    %   %%%%%%%%%%%%%%%%%%%%%%%%%%%%%%%%%%%%%%%%%%%%%%%%%%%%%%%%%%%%%%%%%%%%%%%%%%%%%%%%%%%%%%%%%%%%%%%%%%%%%%%%%%%%%%%%%%%%%%%%%%%%%%%%%%%%%%%%%%%%
                                      & \multirow{3}{*}{\textsc{Fisher}+} 
                                                              & \textcolor{brown}{Accuracy}      & $63.39\rightarrow 63.56$       & $63.39\rightarrow 63.57$       & $63.39\rightarrow 63.57$      \\ 
                                       &                       & \textcolor{cyan}{Weight norm ($\times 10^{-3}$)}    & $12.6 \rightarrow 60.5$   & $12.6 \rightarrow 60.5$   & $12.6 \rightarrow 60.7$ \\
                                       &                       & \textcolor{teal}{Time}           & $1.2$ s   & $1.2$ s   & $1.2$ s \\\cline{2-6} \rule{0pt}{2ex}        
\end{tabular}
}
\vspace{-3mm}
\end{table}
