# Supplementary material for: Efficiently Forgetting What You Have Learned in Graph Representation Learning via Projection
Source: arXiv:2302.08990 source file (2023-02-17)
Supplement: Supplementary file 7 [file logistic_regression_linear_span.tex]

\section{Proof of Proposition~\ref{prop:logistic_regression_linear_span}} \label{appendix:logistic_regression_linear_span}
To see this, let consider a simple case where each column of the weight matrix is initialized as zero vector, i.e., $\mathbf{w}_c(0) = \mathbf{0}$.
Given the objective function as defined in Eq.~\ref{eq:ovr_logistic_regression}, all gradient 
% computed on any node $i$ and at any iteration $t$ is also 
are in the linear span of node feature vectors, i.e.,
\begin{equation}
    \nabla_{\mathbf{w}_c} F_i(\mathbf{W}(t)) = \lambda \mathbf{w}_c(t) + \frac{y_{i,c}}{1+\exp(y_{i,c} \mathbf{w}_c^\top(t) \mathbf{h}_i)} \mathbf{h}_i,~ 
    \mathbf{h}_i = \sum\nolimits_{j=1}^N [\mathbf{P}^L]_{ij} \mathbf{x}_j,
\end{equation}
where $[\mathbf{P}^L]_{ij}$ is the $i$-th row, $j$-th column of $\mathbf{P}^L$.
When training with mini-batch SGD, we have
\begin{equation} \label{eq:mini-batch-sgd}
    \mathbf{w}_c(t+1) = \mathbf{w}_c(t) - \frac{\eta_t}{|\mathcal{B}(t)|} \sum\nolimits_{i \in \mathcal{B}(t)} \nabla_{\mathbf{w}_c} F_i(\mathbf{W}(t)),
\end{equation}
where $\eta_t$ is the learning rate and $\mathcal{B}(t)\subseteq \mathcal{V}_\text{train}$ is the sampled mini-batch at the $t$-th iteration.
Since the gradient satisfies $\nabla_{\mathbf{w}_c} F_i(\mathbf{W}(t)) \in \text{span}\{\mathbf{x}_1, \ldots, \mathbf{x}_N\}$, the weight parameters after $t$-iterations still inside the linear span of node features.
