# Supplementary material for: Efficiently Forgetting What You Have Learned in Graph Representation Learning via Projection
Source: arXiv:2302.08990 source file (2023-02-17)
Supplement: Supplementary file 8 [file svm_linear_span.tex]

\section{Proof of Preposition~\ref{prop:svm_linear_span}} \label{appendix:svm_linear_span}

\begin{equation}\label{eq:svm_primal_dual}
    \begin{aligned}
    f_\text{SVM}(\mathbf{w}) &= \frac{\lambda}{2}\| \mathbf{w}\|_2^2 + \sum_{i=1}^N \max(0, 1-y_i \mathbf{w}^\top \mathbf{x}_i) \\
    g_\text{SVM}(\bm{\alpha}) &= - \frac{1}{2\lambda} \sum_{i=1}^N \sum_{j=1}^N \alpha_i\alpha_j y_i y_j \langle \mathbf{x}_i, \mathbf{x}_j \rangle + \sum_{i=1}^N \alpha_i,~\text{subject to}~\sum_{i=1}^N \alpha_i y_i = 0,~ \alpha_i \in [0, 1]
    \end{aligned}
\end{equation}
